# Supplementary material for: A Novel Model for Vulnerability Analysis through Enhanced Directed Graphs and Quantitative Metrics
Source: arXiv:2112.06453 source file (2021-12-13)
Supplement: Supplementary file 1 [file appendixes.tex]

% =================================================================================
% === XI. Anexos ==================================================================
% =================================================================================
\appendix
\section{Basic Security Definitions}
\label{sec:appendixes}
    In this section, the foundational security concepts of this research work are defined, along with MITRE's, NIST's and FIRST's Common Security Standards, as formal lists or dictionaries supporting security content automation.
    
    \subsection{Industrial Component (IC)}
        According to the ISA/IEC 62443-4-2 standard, an Industrial Component (IC) is one of the parts that make up an industrial product or system, including hardware, software, or other components~\cite{IEC62443}. The ISA/IEC 62443-4-2 document defines four types of components~\cite{IEC62443_4_2}:

            \begin{itemize}
                \item \textbf{Software Application}: One or more software programs and their dependencies\footnote{Any software program that is necessary for the software application to function, such as database packages, reporting tools, or any third party or open source software.} that are used to interface with the process or the control system itself (\textit{e.g.}, configuration software and historian). Software applications typically execute on host devices or embedded devices. 

                \item \textbf{Embedded Device}: Special purpose device designed to directly monitor or control an industrial process (\textit{e.g.}, PLCs, wired or wireless field sensor devices, wired or wireless field actuator devices, safety instrumented system (SIS) controllers, distributed control system (DCS) controllers). According to the ISA/IEC 62443, typical attributes of these devices are limited storage, limited number of exposed services, programmed through an external interface, embedded operating systems (OSs), or firmware equivalent, real-time scheduler, may have an attached control panel, and may have a communications interface.

                \item \textbf{Host Devices}: General purpose device running an operating system (\textit{e.g.}, Microsoft Windows OS or Linux) capable of hosting one or more software applications, data stores or functions from one or more suppliers. This kind of devices typically include attributes such as filesystem, programmable services, no real-time scheduler, and full HMI (keyboard, mouse, etc.).

                \item \textbf{Network Device}: Device that facilitates data flow between devices, or restricts the flow of data, but may not directly interact with a control process. According to the standard, these devices typically include embedded OS or firmware, no HMI, no real-time scheduler, and configured through an external interface.
            \end{itemize}

    \subsection{Weakness}
        Weaknesses are flaws, faults, bugs, and other errors in software and hardware design, architecture, code, or implementation that, if left unaddressed, could result in systems, networks, and hardware being vulnerable to attacks~\cite{CWE1} (\textit{e.g.}, buffer overflow).

    \subsection{Vulnerability}
        A vulnerability is a flaw in a software, firmware, hardware, or service component resulting from a weakness that can be exploited, causing a negative impact to the confidentiality, integrity, or availability of an impacted component or components. It can be used to gain remote or physical access to a system~\cite{CVE_Definitions}. To put it in other words: All vulnerabilities rely on weaknesses, but not all weaknesses entail vulnerabilities.
        
        Vulnerabilities can be classified as both known and unknown~\cite{BasicConcepts_2004}. Known vulnerabilities are those that have been published in publicly available sources such as the National Vulnerability Database (NVD)~\cite{NVD_nist}. On the other hand, unknown vulnerabilities are dormant vulnerabilities that have not been publicly exposed or exploited. These potential vulnerabilities have to be discovered by using other methods such as penetration testing~\cite{commonCriteria_Part3}. In some cases, unknown vulnerabilities might be known for a group of attackers that do not want to disclose their knowledge to take malicious advantages of it (zero-day vulnerabilities)~\cite{zeroDayVulnerabilities_2019}.

    \subsection{Attack Pattern}
        An attack pattern is a description of the common attributes and approaches employed by adversaries to exploit known weaknesses in cyber-enabled capabilities~\cite{CAPEC_Definitions}. Attack patterns define the challenges that an adversary may face and how they go about solving it.

    \subsection{Common Platform Enumeration (CPE) Scheme~\cite{CPE7695, CPE7696, CPE_main}}
        CPE is an abstract structured naming scheme for describing and identifying applications, operating systems, software, and hardware, including industrial control systems, such as Supervisory Control And Data Acquisition (SCADA). The logical construct of a CPE is called ``Well-Formed CPE Name (WFN)''~\cite{CPE7695}. The CPE scheme, however, cannot describe and identify specific instances of products (e.g., using serial numbers, particular licences, or physically discernible products)~\cite{CPE7696}. CPE is operated by the NIST~\cite{nist}. The latest version at the time this paper was written is version 2.3.

        Version 8.0.6001 of Internet Explorer for its \textit{beta} update can be represented using version 2.3 of the CPE naming specification\footnote{\textit{cpe:2.3:a:microsoft:internet\_explorer:8.0.6001:beta:*:*:*:*:*:*}}. The ``\textit{a}'' after the CPE version indicates that the following element is a software application.

    \subsection{Common Weakness Enumeration (CWE)~\cite{CWE0, CWE1}}
        CWE is a community-developed list of common software and hardware weakness types, each one associated with some CVEs (explained in the next subsection). CWE is operated by the MITRE Corporation~\cite{mitreCorporation}. The latest version at the time this paper was written is version 4.3.

        CWE-119 is an example of a weakness present in all updates of version 8 of Internet Explorer. It is related to improper restriction of operations within the bounds of a memory buffer.

    \subsection{Common Vulnerabilities and Exposures (CVE)~\cite{CVE1, CVE2, CWE1}}
        CVE is a list of common identifiers for publicly known cybersecurity vulnerabilities~\cite{CVE1} operated by the MITRE Corporation~\cite{mitreCorporation}. Each CVE includes a unique identification number, a description, one public reference, a reference to the software or hardware that is affected (using CPE), a reference to a weakness, and its severity~\cite{ARES}. As Dimitriadis \textit{et al.} state in~\cite{ARES}, ``it can be assumed that CVEs are ``known knowns'' (things we are aware of and understand) or specific vulnerabilities, while CWEs are ``unknown knowns'' (things we understand but are not aware of) or generic vulnerability types.'' The latest CVE version is always available in its official site\footnote{https://cve.mitre.org/}.
        
        CVE-2015-6154 is an example of a vulnerability that exploits the CWE-119 weakness present in Internet Explorer 8, allowing remote attackers to execute arbitrary code or cause a denial of service (memory corruption) via a crafted website.

    \subsection{Common Vulnerability Scoring System (CVSS)~\cite{CVSS1, CVE2}}
        CVSS is a public framework that provides a standardized method for assigning quantitative values (scores) to security vulnerabilities (CVE)~\cite{CVE2} according to their severity~\cite{CVSS1}. A CVSS score is a decimal number in the range [0.0, 10.0]. The latest version at the time this paper was written is version 3.1.
        
        The CVSS value for vulnerability CVE-2015-6154 is $9.3$ out of $10$. This value is classified as critical.

    \subsection{Common Attack Pattern Enumeration and Classification (CAPEC)~\cite{CAPEC1, ARES}}
        CAPEC is a comprehensive dictionary that provides a publicly available classification taxonomy of known attack patterns (security threats)~\cite{CAPEC1}. In~\cite{ARES}, Dimitriadis \textit{et al.} explain that each CAPEC describes the common characteristics of a cyber threat (aka attack-pattern), helping to explain how applications and other cyber-enabled capabilities are likely to be attacked. CAPEC also provides the likelihood that the attack pattern can occur and its impact. CAPEC utilizes a qualitative approach, rating both likelihood and impact in a five-step value scale ranging from very low to very high. Finally, each CAPEC records the weaknesses (CWEs) that the attack pattern can exploit. The latest version at the time this article was written is version 3.4.
    
    \subsection{System Under Test (SUT)}
        The System Under Test (SUT) is defined as a system such as a Control System (CS), SCADA system or Monitoring System that is available from a single system supplier~\cite{commonCriteriaGeneralModel}. A SUT may be comprised of hardware and software components from several manufacturers but must be integrated into a single system and supported, as a whole, by a single supplier. The SUT may be an IC, a part of an IC, a set of ICs, a unique technology that may never be made into a product, or a combination of these.
